# Supplementary material for: On the Practicality of Deterministic Epistemic Uncertainty
Source: arXiv:2107.00649 source file (2022-07-05)
Supplement: Supplementary file 1 [file cifar10_regularization_strength.tex]

\begin{figure}[t]
\centering
\setlength{\tabcolsep}{-7pt}
\resizebox{1.1\linewidth}{!}{
\begin{tabular}{cccc}
% \vspace{-4mm}
% \hspace{-3mm}
\input{figures/image_classification/regularization_strength/dropout_cifar10_AULC_additive_gaussian_vs_ACC} & \hspace{1mm}
\input{figures/image_classification/regularization_strength/dropout_cifar10_AULC_jpeg_quality_vs_ACC} & 
\input{figures/image_classification/regularization_strength/dropout_cifar10_stl10_AUROC_vs_ACC}  & \hspace{-6mm}
\input{figures/image_classification/regularization_strength/dropout_cifar10_svhn_cropped_AUROC_vs_ACC} 
\\ \vspace{-1mm}
\input{figures/image_classification/regularization_strength/duq_cifar10_AULC_additive_gaussian_vs_ACC} &  \hspace{1mm}
\input{figures/image_classification/regularization_strength/duq_cifar10_AULC_jpeg_quality_vs_ACC} & \hspace{0mm}
\input{figures/image_classification/regularization_strength/duq_cifar10_stl10_AUROC_vs_ACC}  & \hspace{1mm}
\input{figures/image_classification/regularization_strength/duq_cifar10_svhn_cropped_AUROC_vs_ACC}
\\ \vspace{-1mm}
\input{figures/image_classification/regularization_strength/sngp_cifar10_AULC_additive_gaussian_vs_ACC} &  \hspace{1mm}
\input{figures/image_classification/regularization_strength/sngp_cifar10_AULC_jpeg_quality_vs_ACC} & 
\input{figures/image_classification/regularization_strength/sngp_cifar10_stl10_AUROC_vs_ACC}  & \hspace{-6mm}
\input{figures/image_classification/regularization_strength/sngp_cifar10_svhn_cropped_AUROC_vs_ACC}
\\ \vspace{-1mm}
\input{figures/image_classification/regularization_strength/mir_cifar10_AULC_additive_gaussian_vs_ACC} & \hspace{1mm}
\input{figures/image_classification/regularization_strength/mir_cifar10_AULC_jpeg_quality_vs_ACC} & \hspace{1mm}
\input{figures/image_classification/regularization_strength/mir_cifar10_stl10_AUROC_vs_ACC}  & \hspace{-6mm}
\input{figures/image_classification/regularization_strength/mir_cifar10_svhn_cropped_AUROC_vs_ACC}  
\\ \vspace{-1mm}
\end{tabular}
}
\vspace{-0.5em}
\caption{Trained on CIFAR10. Vertical axis: Test accuracy. Horizontal axis: \ac{raulc} against additive gaussian noise (1st column) and additive jpeg quality corruption (2nd column), \ac{auroc} against STL10 (3rd column) and SVHN (4th column) for Dropout (1st row), DUQ (2nd row), SNGP (3rd row) and MIR (4th row) using different regularization strength. For SNGP a larger hyperparameter corresponds to less regularization. For Dropout we observe a correlation between regularization strength and performance.}\label{fig:suppl_cifar_sensitivity_to_regularization_strength}
\vspace{-1em}
\end{figure}
