# Supplementary material for: On the Practicality of Deterministic Epistemic Uncertainty
Source: arXiv:2107.00649 source file (2022-07-05)
Supplement: Supplementary file 3 [file cifar_10_100_c_supplement.tex]

\begin{table}[!h]
\centering
\begin{tabular}{c | c c c | c c c}
    \toprule
            Method & & CIFAR10-C & & CIFAR100-C & \\
            & ACC & AUROC & rAULC & ACC & AUROC & rAULC\\
            \midrule
            Softmax & 0.882 $\pm$ 0.008 & 0.782 $\pm$ 0.04 & 0.708 $\pm$ 0.069  & 0.61 $\pm$ 0.042 & 0.762 $\pm$ 0.013 & 0.596 $\pm$ 0.037 \\ 
            MC Dropout~\cite{gal2016dropout} & 0.885 $\pm$ 0.001 & 0.866 $\pm$ 0.023 & 0.829 $\pm$ 0.036 & 0.615 $\pm$ 0.001 & 0.818 $\pm$ 0.01 & 0.726 $\pm$ 0.024 \\  
            Ensemble~\cite{lakshminarayanan2017simple} & 0.91 $\pm$ 0.008 & 0.85 $\pm$ 0.041 & 0.833 $\pm$ 0.069 & 0.628 $\pm$ 0.042 & 0.824 $\pm$ 0.012 & 0.713 $\pm$ 0.031 \\ 
            \midrule
            SNGP~\cite{liu2020simple} & 0.903 $\pm$ 0.0 & 0.833 $\pm$ 0.04 & 0.766 $\pm$ 0.073 & 0.611 $\pm$ 0.0 & 0.788 $\pm$ 0.009 & 0.623 $\pm$ 0.02 \\ 
            DDU~\cite{mukhoti2021deterministic} & 0.884 $\pm$ 0.0 & 0.673 $\pm$ 0.057 & 0.441 $\pm$ 0.155 & 0.609 $\pm$ 0.0 & 0.635 $\pm$ 0.021 & 0.339 $\pm$ 0.053 \\
            MIR~\cite{postels2020hidden} & 0.889 $\pm$ 0.0 & 0.79 $\pm$ 0.04 & 0.697 $\pm$ 0.078 & 0.617 $\pm$ 0.0 & 0.726 $\pm$ 0.018 & 0.514 $\pm$ 0.034 \\ 
            DUQ~\cite{van2020uncertainty} & 0.86 $\pm$ 0.0 & 0.773 $\pm$ 0.068 & 0.614 $\pm$ 0.154 & - & - & - \\
            DCU~\cite{winkens2020contrastive} & 0.945 $\pm$ 0.0 & 0.794 $\pm$ 0.037 & 0.706 $\pm$ 0.06 & 0.642 $\pm$ 0.0 & 0.75 $\pm$ 0.053 & 0.558 $\pm$ 0.099 \\
     \bottomrule
\end{tabular}
\end{table}
