# Supplementary material for: On the Practicality of Deterministic Epistemic Uncertainty
Source: arXiv:2107.00649 source file (2022-07-05)
Supplement: Supplementary file 4 [file cityscapes_c_carla_supplement.tex]

\begin{table}[!h]
\centering
\begin{tabular}{c | c c c | c c c}
    \toprule
            Method & & Cityscapes & & & CARLA & \\
             & mIoU & AUROC & rAULC & mIoU & AUROC & rAULC\\
            \midrule
            Softmax & 0.503 $\pm$ 0.003 & 0.815 $\pm$ 0.076 & 0.737 $\pm$ 0.138 & 0.422 $\pm$ 0.015 & 0.854 $\pm$ 0.028 & 0.818 $\pm$ 0.033 \\ 
            MC Dropout~\cite{gal2016dropout} & 0.506 $\pm$ 0.011 & 0.846 $\pm$ 0.034 & 0.785 $\pm$ 0.081 & 0.41 $\pm$ 0.049 & 0.843 $\pm$ 0.004 & 0.73 $\pm$ 0.017 \\  
            Ensemble~\cite{lakshminarayanan2017simple} & 0.525 $\pm$ 0.010 & 0.835 $\pm$ 0.041 & 0.751 $\pm$ 0.079 & 0.428 $\pm$ 0.03 & 0.863 $\pm$ 0.012 & 0.812 $\pm$ 0.012 \\ 
            \midrule
            SNGP~\cite{liu2020simple} & 0.519 $\pm$ 0.002 & 0.833 $\pm$ 0.047 & 0.759 $\pm$ 0.103 & 0.424 $\pm$ 0.038 & 0.853 $\pm$ 0.031 & 0.813 $\pm$ 0.041 \\
            DDU~\cite{mukhoti2021deterministic} & 0.505 $\pm$ 0.005 & 0.731 $\pm$ 0.029 & 0.542 $\pm$ 0.053 & 0.408 $\pm$ 0.042 & 0.467 $\pm$ 0.014 & -0.038 $\pm$ 0.015 \\ 
            MIR~\cite{postels2020hidden} & 0.504 $\pm$ 0.005 & 0.729 $\pm$ 0.033 & 0.564 $\pm$ 0.062 & 0.412 $\pm$ 0.012 & 0.744 $\pm$ 0.009 & 0.619 $\pm$ 0.031 \\
     \bottomrule
\end{tabular}
\caption{Cityscapes.}
\end{table}
