# Supplementary material for: On the Practicality of Deterministic Epistemic Uncertainty
Source: arXiv:2107.00649 source file (2022-07-05)
Supplement: Supplementary file 5 [file minimal_shift_uncertainty_old.tex]

\begin{figure}[t]
\centering
\setlength{\tabcolsep}{3pt}
\setlength{\aboverulesep}{0pt}
\setlength{\belowrulesep}{0pt}
% \renewcommand{\arraystretch}{3}
% \resizebox{1.1\linewidth}{!}{
\begin{tabular}{cccccc}
% \vspace{-4mm}
% \hspace{-3mm}
 & Input & GT & Prediction & Error & Uncertainty \\
\hline\addlinespace[2pt]
\multirow{2}{*}{\rotatebox[origin=c]{90}{Softmax}} &
% \\[\dimexpr-\normalbaselineskip+2pt] &
\includegraphics[width=2.5cm,trim={2.1cm 2.15cm 1.65cm 2.5cm},clip]{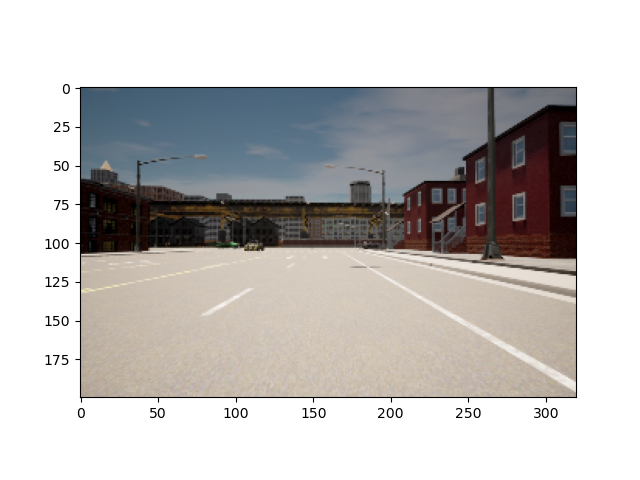} & 
\includegraphics[width=2.5cm,trim={2.1cm 2.15cm 1.65cm 2.5cm},clip,trim={2.1cm 2.15cm 1.65cm 2.5cm},clip]{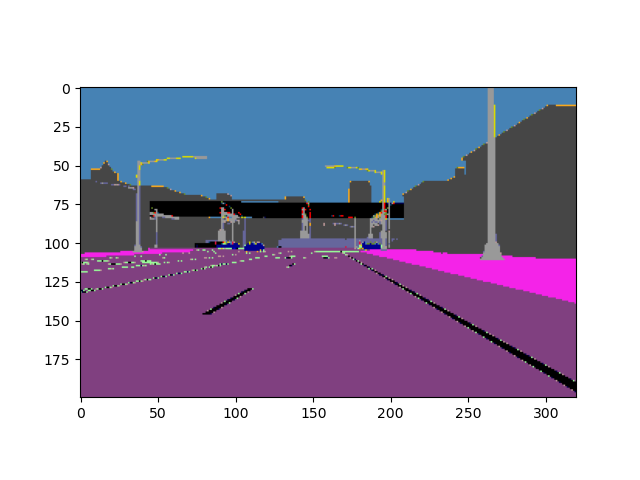} & 
\includegraphics[width=2.5cm,trim={2.1cm 2.15cm 1.65cm 2.5cm},clip]{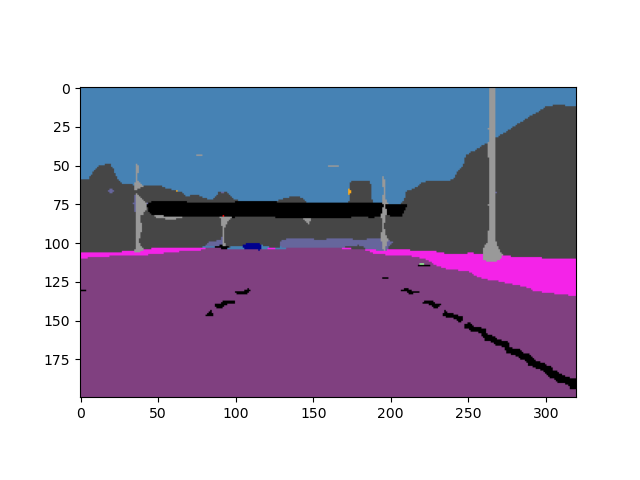} &
\includegraphics[width=2.5cm,trim={2.1cm 2.15cm 1.65cm 2.5cm},clip]{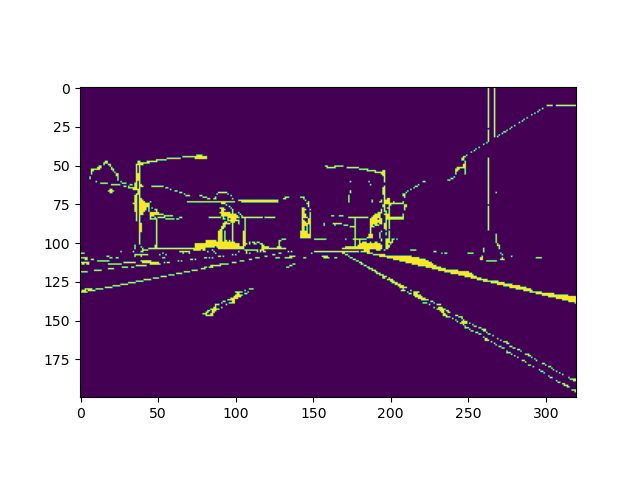} &
\includegraphics[width=2.5cm,trim={2.1cm 2.15cm 1.65cm 2.5cm},clip]{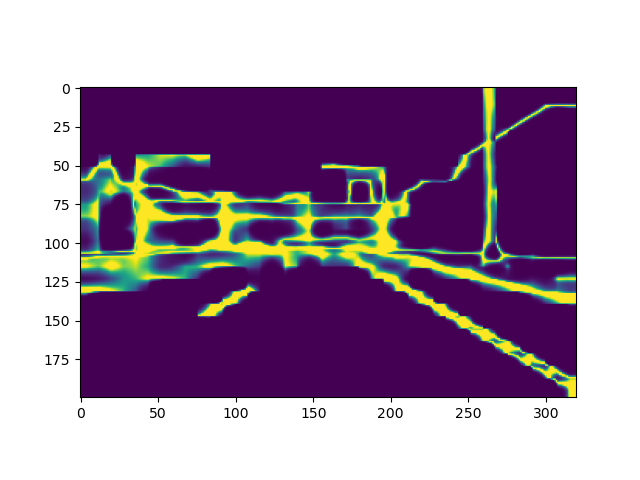} 
\\ 
& 
% \\[\dimexpr-\normalbaselineskip+2pt] &
\includegraphics[width=2.5cm,trim={2.1cm 2.15cm 1.65cm 2.5cm},clip]{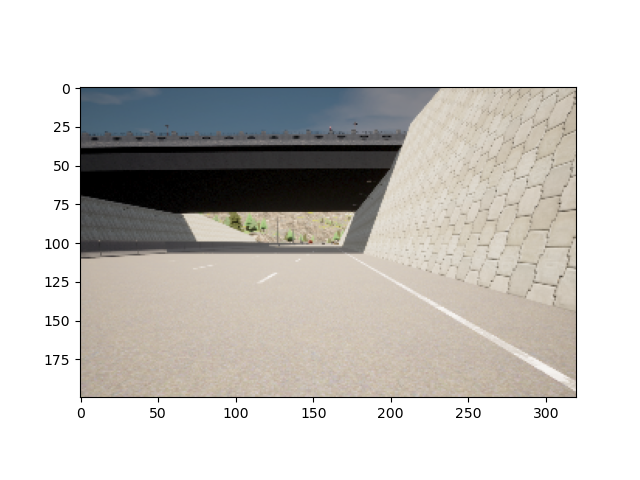} & 
\includegraphics[width=2.5cm,trim={2.1cm 2.15cm 1.65cm 2.5cm},clip,trim={2.1cm 2.15cm 1.65cm 2.5cm},clip]{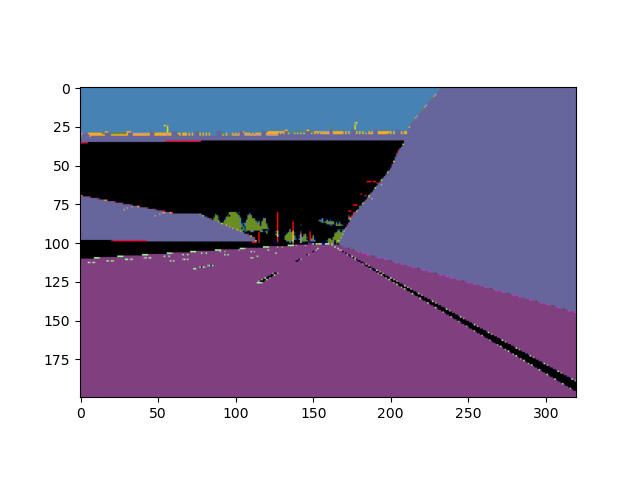} & 
\includegraphics[width=2.5cm,trim={2.1cm 2.15cm 1.65cm 2.5cm},clip]{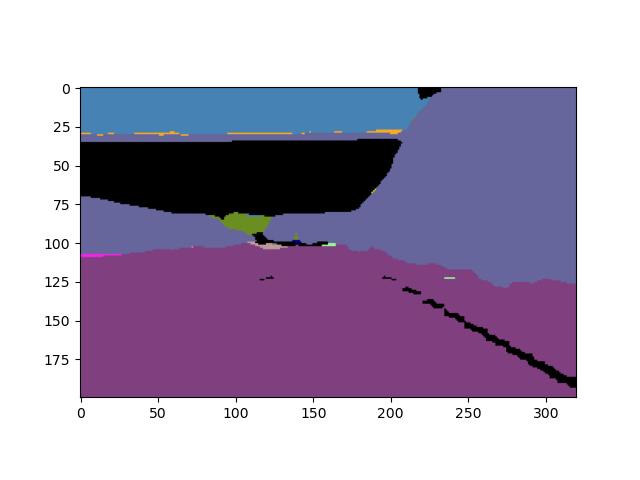} &
\includegraphics[width=2.5cm,trim={2.1cm 2.15cm 1.65cm 2.5cm},clip]{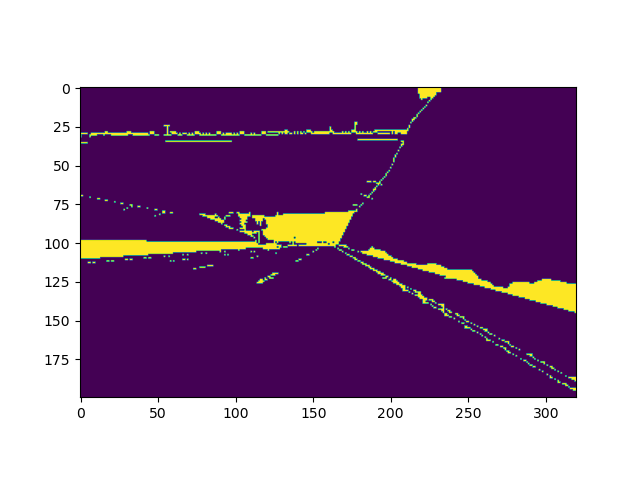} &
\includegraphics[width=2.5cm,trim={2.1cm 2.15cm 1.65cm 2.5cm},clip]{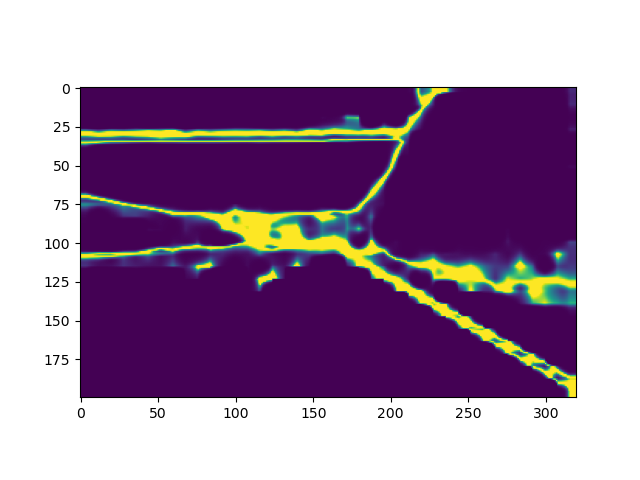} 
\\
\hline\addlinespace[2pt]
\multirow{2}{*}{\rotatebox[origin=c]{90}{Dropout}} &
\includegraphics[width=2.5cm,trim={2.1cm 2.15cm 1.65cm 2.5cm},clip]{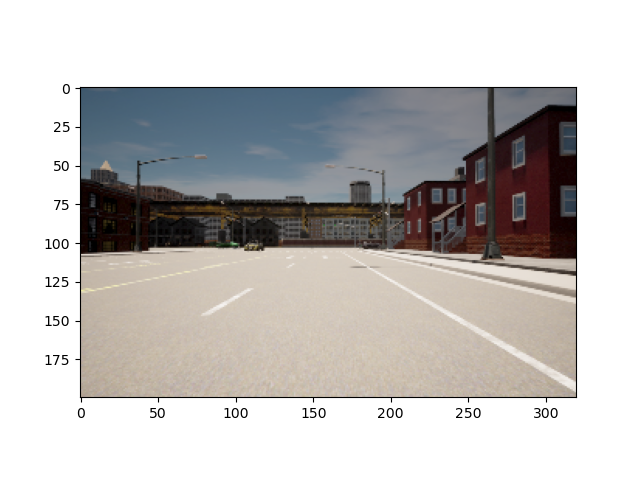} & 
\includegraphics[width=2.5cm,trim={2.1cm 2.15cm 1.65cm 2.5cm},clip,trim={2.1cm 2.15cm 1.65cm 2.5cm},clip]{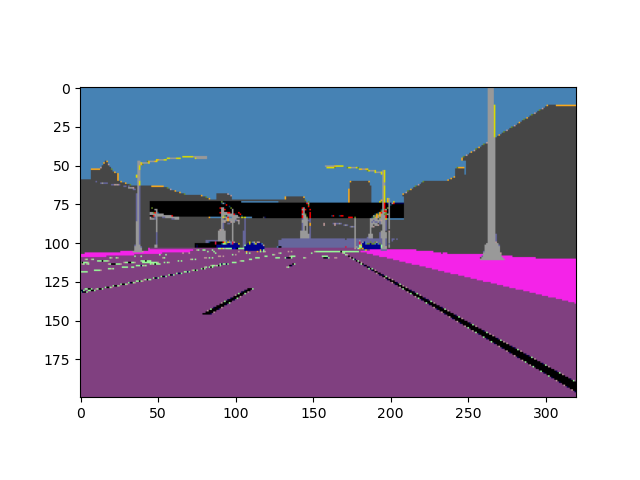} & 
\includegraphics[width=2.5cm,trim={2.1cm 2.15cm 1.65cm 2.5cm},clip]{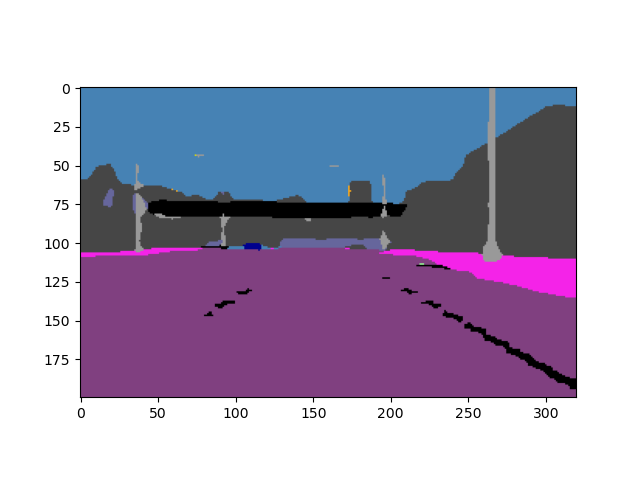} &
\includegraphics[width=2.5cm,trim={2.1cm 2.15cm 1.65cm 2.5cm},clip]{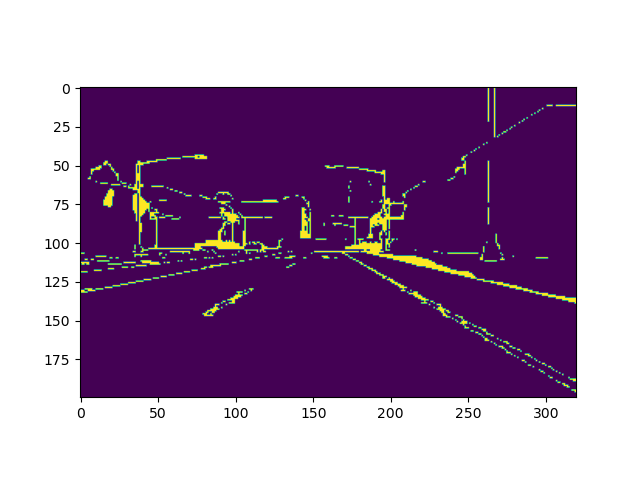} &
\includegraphics[width=2.5cm,trim={2.1cm 2.15cm 1.65cm 2.5cm},clip]{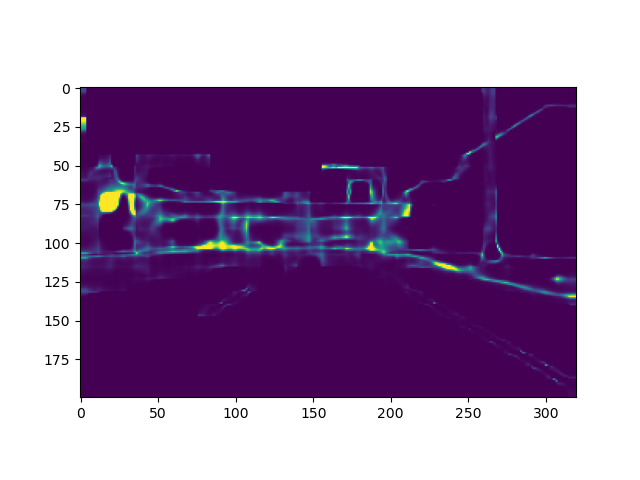} 
\\
& 
\includegraphics[width=2.5cm,trim={2.1cm 2.15cm 1.65cm 2.5cm},clip]{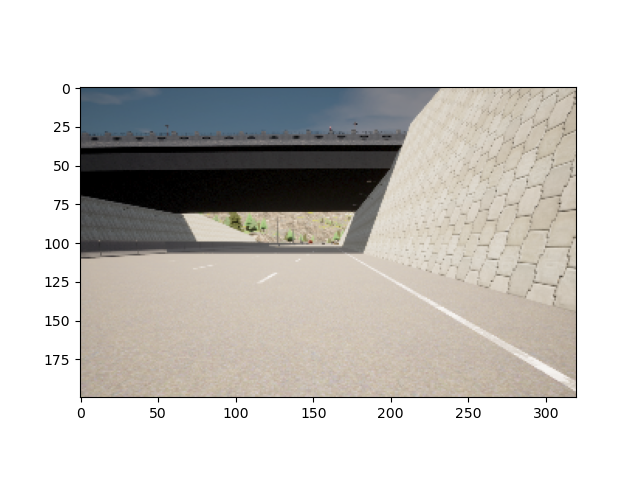} & 
\includegraphics[width=2.5cm,trim={2.1cm 2.15cm 1.65cm 2.5cm},clip,trim={2.1cm 2.15cm 1.65cm 2.5cm},clip]{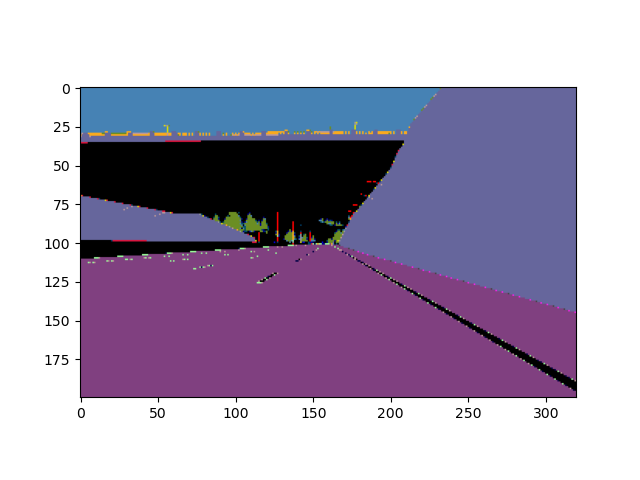} & 
\includegraphics[width=2.5cm,trim={2.1cm 2.15cm 1.65cm 2.5cm},clip]{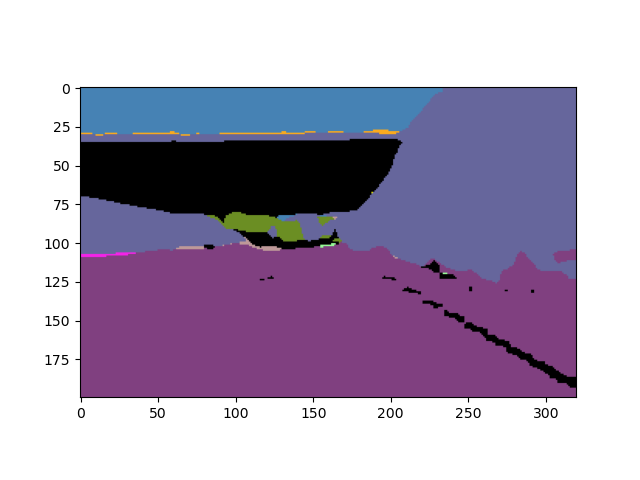} &
\includegraphics[width=2.5cm,trim={2.1cm 2.15cm 1.65cm 2.5cm},clip]{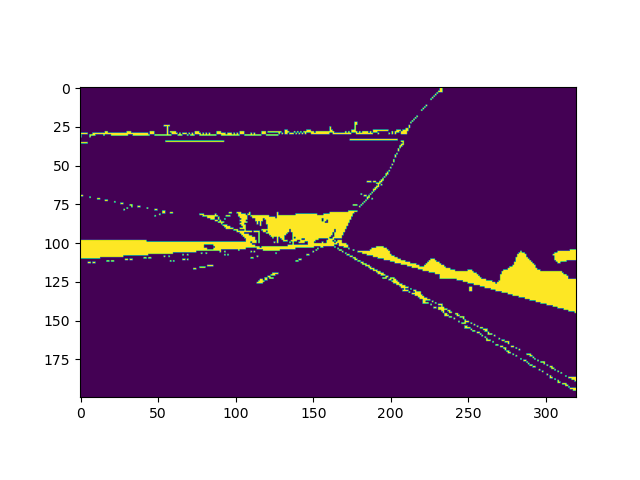} &
\includegraphics[width=2.5cm,trim={2.1cm 2.15cm 1.65cm 2.5cm},clip]{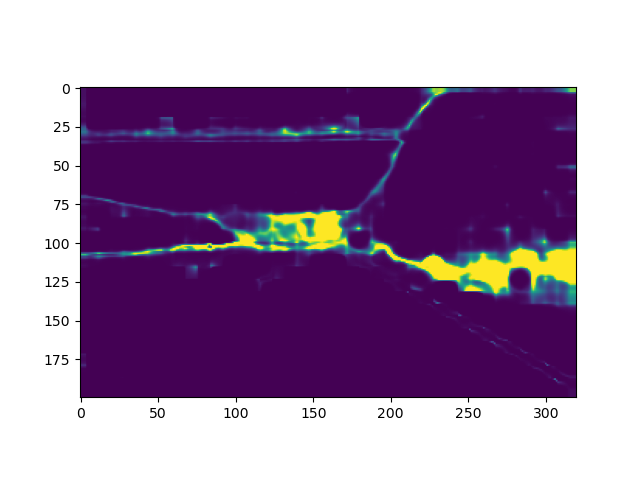} 
\\
\hline\addlinespace[2pt]
\multirow{2}{*}{\rotatebox[origin=c]{90}{SNGP}} &
\includegraphics[width=2.5cm,trim={2.1cm 2.15cm 1.65cm 2.5cm},clip]{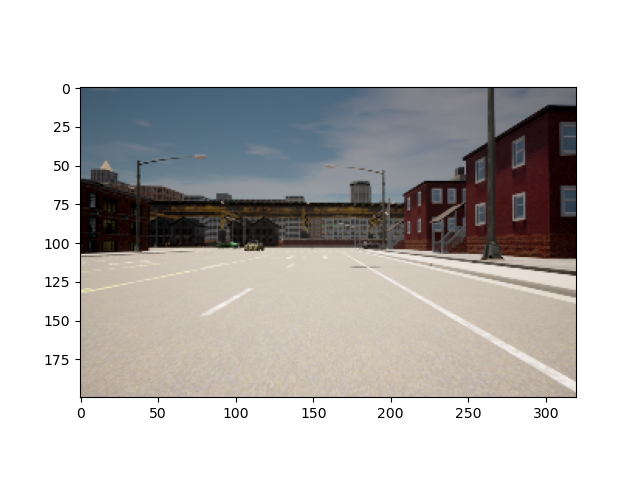} & 
\includegraphics[width=2.5cm,trim={2.1cm 2.15cm 1.65cm 2.5cm},clip,trim={2.1cm 2.15cm 1.65cm 2.5cm},clip]{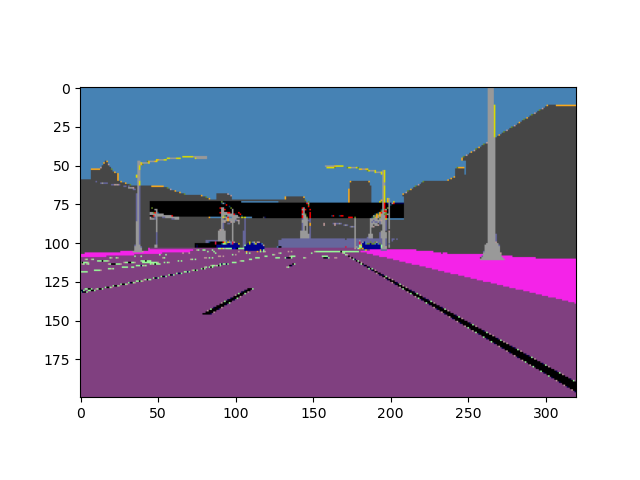} & 
\includegraphics[width=2.5cm,trim={2.1cm 2.15cm 1.65cm 2.5cm},clip]{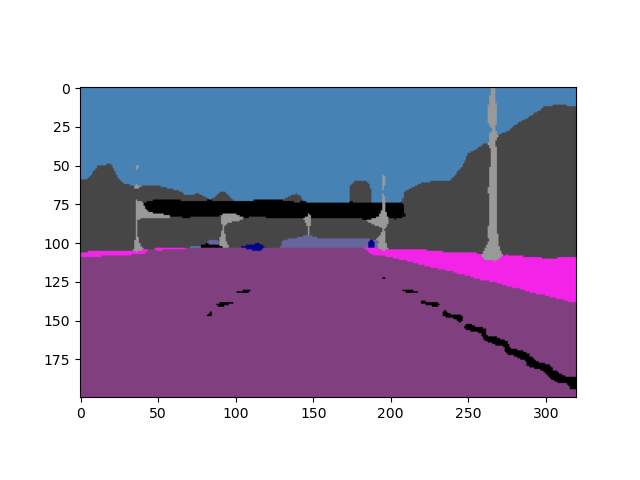} &
\includegraphics[width=2.5cm,trim={2.1cm 2.15cm 1.65cm 2.5cm},clip]{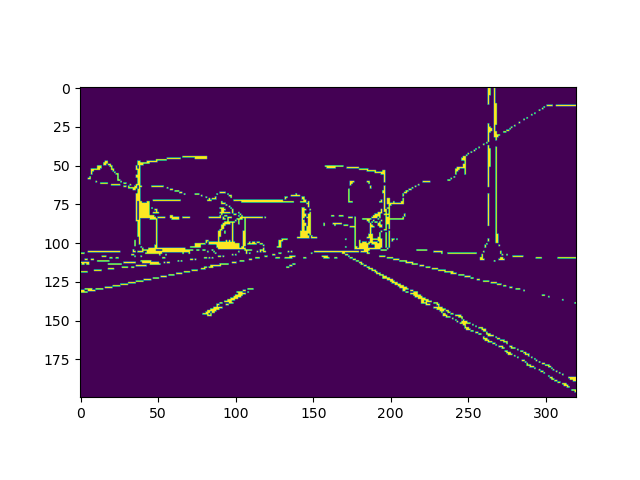} &
\includegraphics[width=2.5cm,trim={2.1cm 2.15cm 1.65cm 2.5cm},clip]{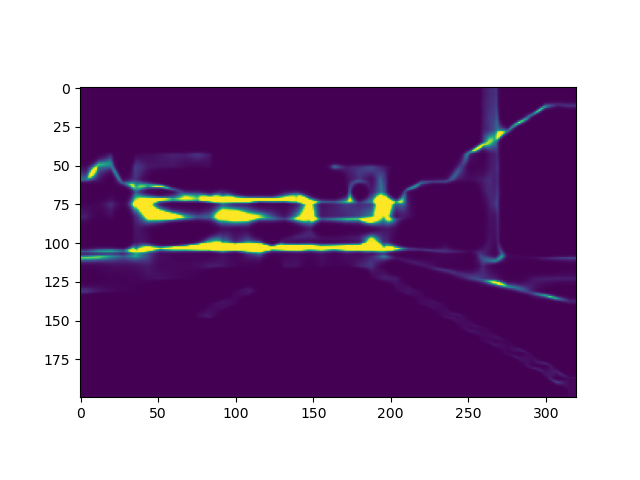} 
\\
& 
\includegraphics[width=2.5cm,trim={2.1cm 2.15cm 1.65cm 2.5cm},clip]{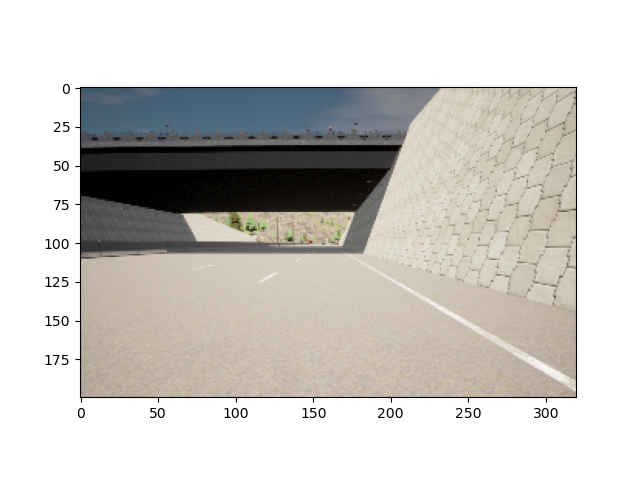} & 
\includegraphics[width=2.5cm,trim={2.1cm 2.15cm 1.65cm 2.5cm},clip,trim={2.1cm 2.15cm 1.65cm 2.5cm},clip]{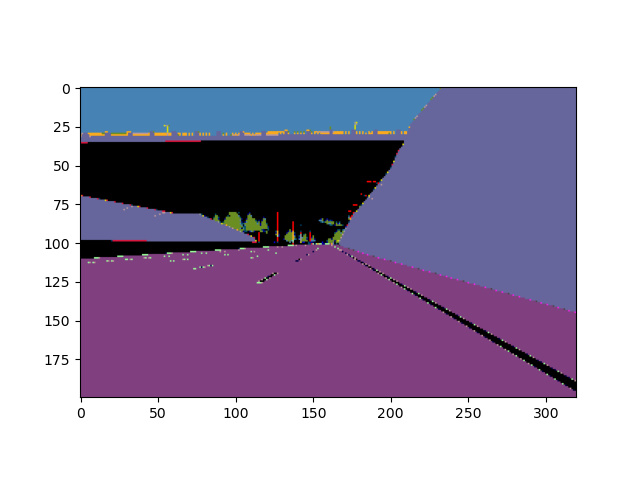} & 
\includegraphics[width=2.5cm,trim={2.1cm 2.15cm 1.65cm 2.5cm},clip]{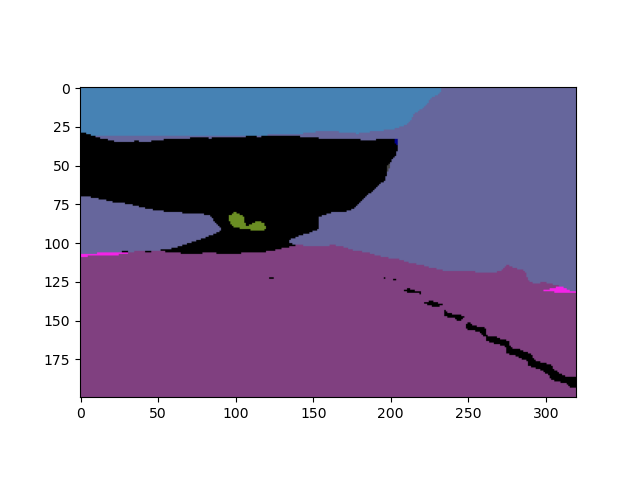} &
\includegraphics[width=2.5cm,trim={2.1cm 2.15cm 1.65cm 2.5cm},clip]{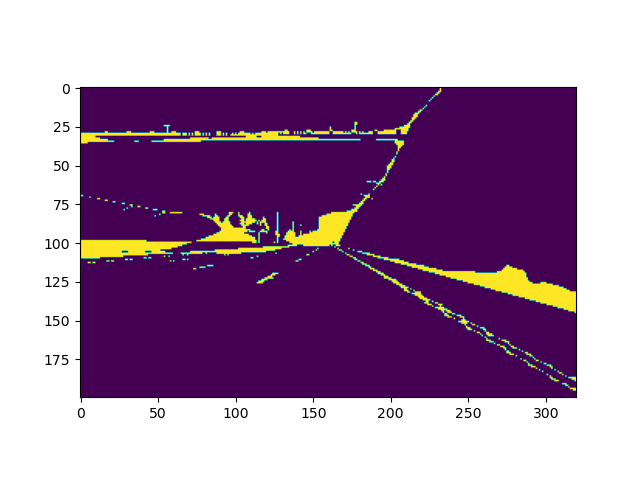} &
\includegraphics[width=2.5cm,trim={2.1cm 2.15cm 1.65cm 2.5cm},clip]{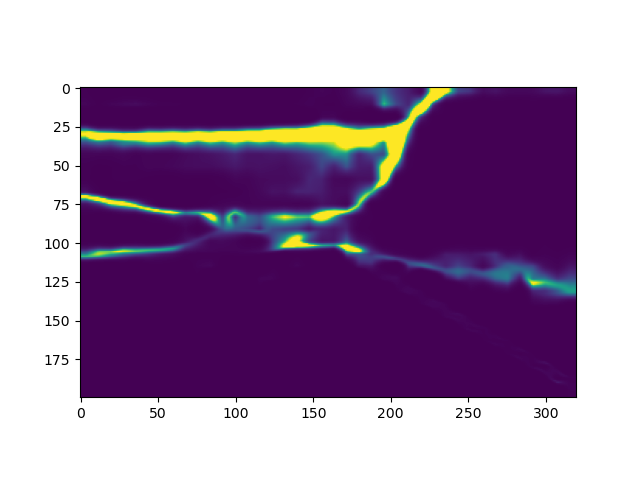} 
\\
\hline\addlinespace[2pt]
\multirow{2}{*}{\rotatebox[origin=c]{90}{MIR}} & 
\includegraphics[width=2.5cm,trim={2.1cm 2.15cm 1.65cm 2.5cm},clip]{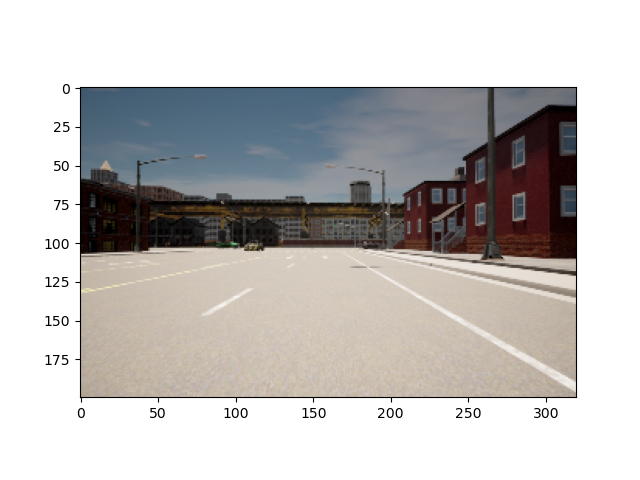} & 
\includegraphics[width=2.5cm,trim={2.1cm 2.15cm 1.65cm 2.5cm},clip,trim={2.1cm 2.15cm 1.65cm 2.5cm},clip]{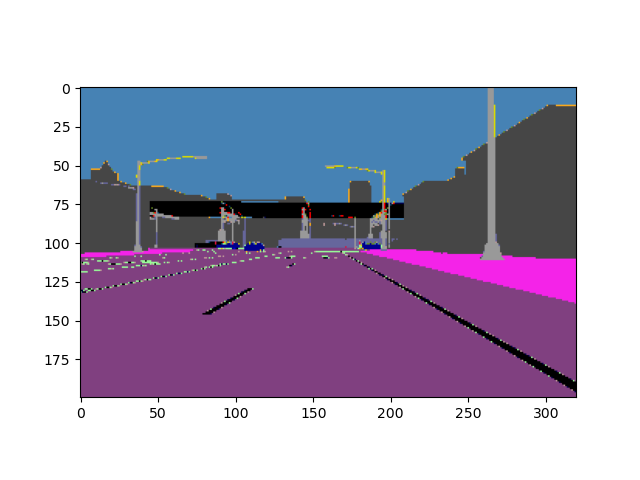} & 
\includegraphics[width=2.5cm,trim={2.1cm 2.15cm 1.65cm 2.5cm},clip]{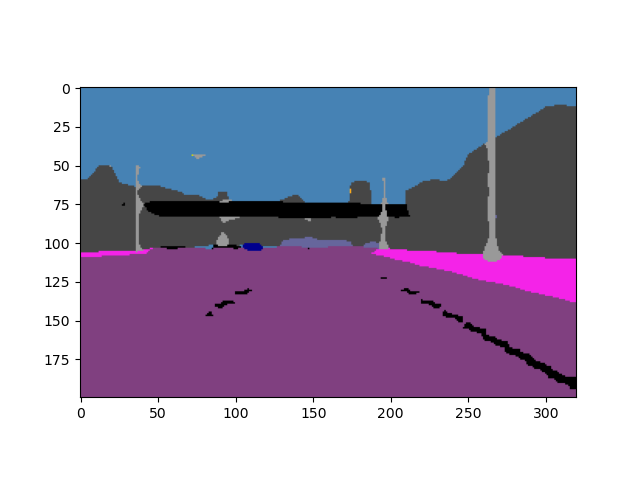} &
\includegraphics[width=2.5cm,trim={2.1cm 2.15cm 1.65cm 2.5cm},clip]{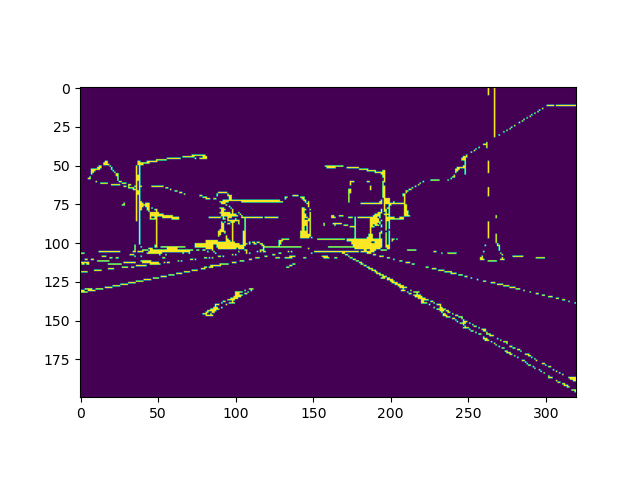} &
\includegraphics[width=2.5cm,trim={2.1cm 2.15cm 1.65cm 2.5cm},clip]{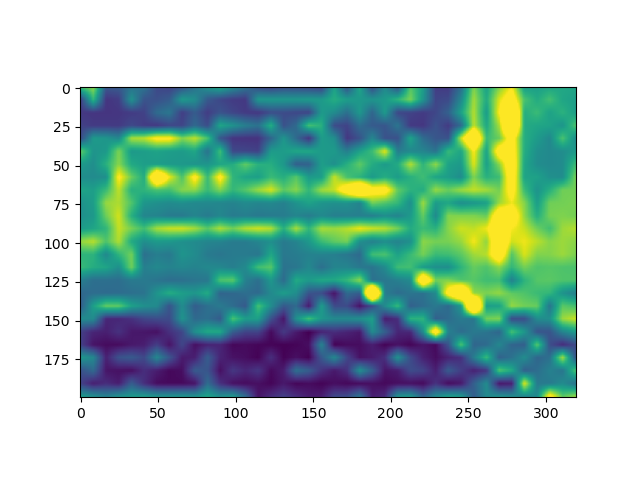} 
\\
& 
\includegraphics[width=2.5cm,trim={2.1cm 2.15cm 1.65cm 2.5cm},clip]{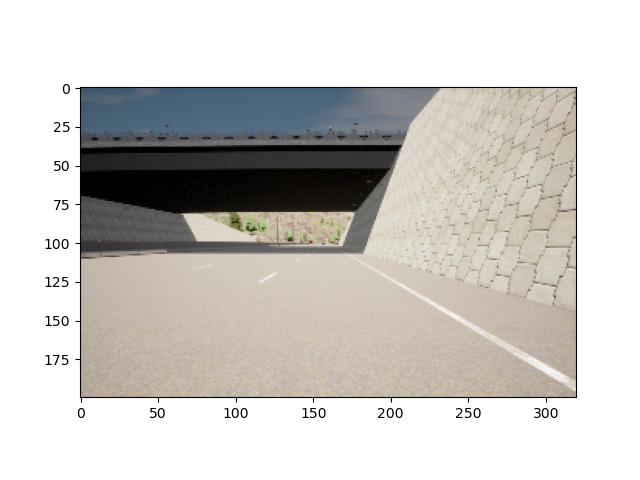} & 
\includegraphics[width=2.5cm,trim={2.1cm 2.15cm 1.65cm 2.5cm},clip,trim={2.1cm 2.15cm 1.65cm 2.5cm},clip]{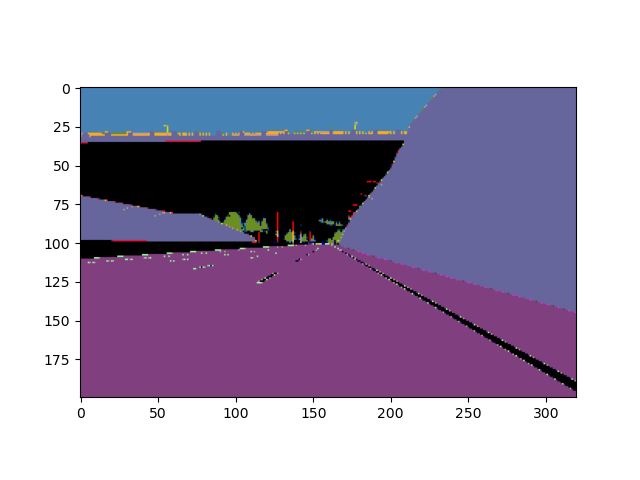} & 
\includegraphics[width=2.5cm,trim={2.1cm 2.15cm 1.65cm 2.5cm},clip]{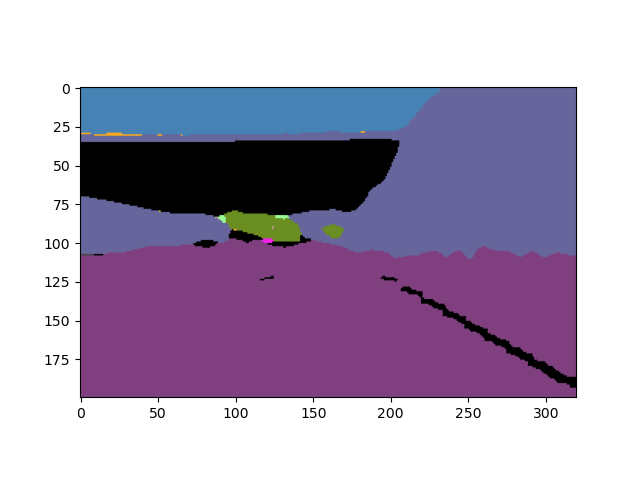} &
\includegraphics[width=2.5cm,trim={2.1cm 2.15cm 1.65cm 2.5cm},clip]{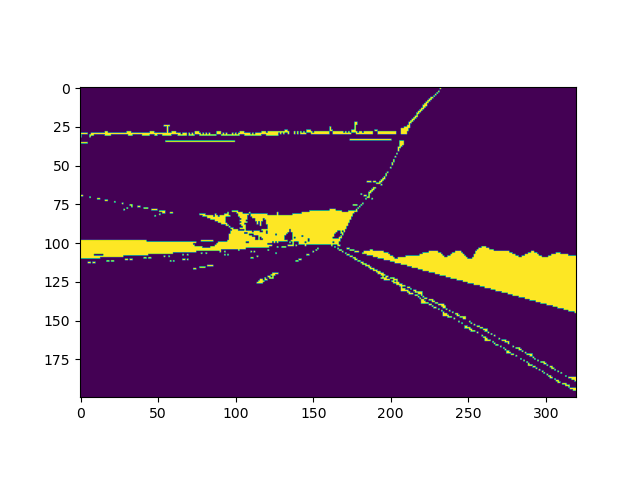} &
\includegraphics[width=2.5cm,trim={2.1cm 2.15cm 1.65cm 2.5cm},clip]{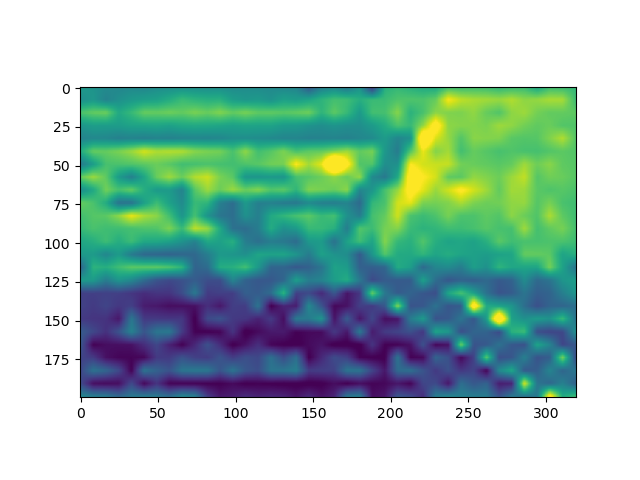} 
\\
\end{tabular}
% }
\vspace{-0.5em}
\caption{Minimal distribution shift.}\label{fig:suppl_segmentation_85
}
\vspace{-1em}
\end{figure}
